# Supplementary material for: Adjustable Robust Nonlinear Network Design Without Controllable Elements under Load Scenario Uncertainties
Source: arXiv:2405.17867 source file (2025-01-17)
Supplement: Supplementary file 1 [file appendix-detailed-example.tex]

\section{Detailed Explanation of the Example in Section~5}
\label{sec:appendix-explanation-example}

In the first iteration, for one of the node pairs~$(\node,
\otherNode)$ with~$\otherNode \in \exits$, we add the worst-case
scenario~$\loadFlowVec \in U$ given by~$\loadFlowVec_{\node} =
\loadFlowVec_{\otherNode}= 2$ and the remaining demands are zero.
The corresponding flows~$\massflow$ are given
by~$\massflow_{(\node,0)}=\massflow_{(0, \otherNode)}=2$ and the
remaining flows are zero.
Further, we set the potentials~$\potential_{\node} = 8, \,
\potential_{\otherNode} = 0,$ and the remaining potentials have
value~$4$.
We note that these potentials do not have to satisfy any
potential bounds in the adversarial
problem~(\ref{eq:maximum-potential-difference}).
The point~$(\loadFlowVec, \massflow, \potential)$ is a solution
of the adversarial
problem~(\ref{eq:maximum-potential-difference})
\wrt~$(\node,\otherNode)$ with objective value~$8$ and, thus,
violates the corresponding potential
bounds~$8 > 4=5-1=\ubPot_{\node}-\lbPot_{\otherNode}$.
We note that this potential drop is maximal since for each arc of the
unique path from~$u$ to~$v$ the flow is maximal \wrt~$U$ and the
potential function is strictly increasing.
Solving the network expansion MINLP~(\ref{expansion})
\wrt~$S=\set{\loadFlowVec}$ leads to the
expansion decisions~$\expVar_{(\node,0,\text{ca})} =
\expVar_{(0,\otherNode,\text{ca})}=1$, \ie, we expand the capacity
along the unique path from~$\node$ to $\otherNode$; see
Figure~\ref{fig:network-worst-case-scenario-example-B} in which
w.l.o.g.~$v=1$ is assumed.
In the expanded network, the previous worst-case scenario is now
feasible.
However, for each other node pair~$(\node,w)$ with $w \in \exits
\setminus \set{\otherNode}$, the worst-case
scenario with the same structure, \ie,
$\tilde{\loadFlowVec}_{\node}=\tilde{\loadFlowVec}_{w}=2$ and the
remaining demands
are zero, is infeasible.
Further, this scenario can again be extended to a solution of the
adversarial problem~(\ref{eq:maximum-potential-difference})
\wrt~$(\node,w)$ in the expanded network and
has an objective value of~$5$, which violates the
corresponding potential bounds.
Adding this scenario to the worst-case uncertainty set implies that
the candidate arc~$(\node,w,\text{ca})$ has to be \rev{build}, \ie,
$\expVar_{(\node,w,\text{ca})} = 1$.
Consequently, in the following iterations of
Algorithm~\ref{alg:adversarial-approach}, we add for each node
pair~$(\node,w)$ with $w \in \exits$ the corresponding worst-case
scenario with the previously described structure.
Thus, Algorithm~\ref{alg:adversarial-approach} terminates after
$n$~iterations with a robust  network, in which every candidate arc is
built; see Figure~\ref{fig:network-worst-case-scenario-example-C}.
To obtain this robust network, the algorithm considered the following
set of demand scenarios
\begin{equation*}
  S = \set{\loadFlowVec_{\node} = \loadFlowVec_{\otherNode}=2, \
    \loadFlowVec_{w} = 0, w \in \exits \setminus \set{\otherNode}
    \forAll
    \otherNode \in \exits},
\end{equation*}
which has a cardinality of~$\abs{\exits}$.
Consequently, the number of worst-case scenarios scales
with the number of sinks in the considered network.
